# Supplementary material for: Quantum dots formed in three-dimensional Dirac semimetal Cd$_3$As$_2$ nanowires
Source: arXiv:1812.06416 source file (2018-12-16)
Supplement: Supplementary file 1 [file Supporting_Information_MinkyungJung.pdf]

# Supporting Information:

# Quantum dots formed in three-dimensional Dirac semimetal $Cd_3As_2$ nanowires

Minkyung Jung,[*,†] Kenji Yoshida,[‡] Kidong Park,[¶] Xiao-Xiao Zhang,[§] Can Yesilyurt,[||] Zhuo Bin Siu,[||] Mansoor B. A. Jalil,[||] Jinwan Park,[⊥] Jeunghee Park,[¶] Naoto Nagaosa,[§,#] Jungpil Seo,[*,⊥] and Kazuhiko Hirakawa[*,‡,@]

† *DGIST Research Institute, DGIST, 333 TechnoJungang, Hyeongpung, Daegu 42988, Korea*

‡ *Center for Photonics Electronics Convergence, IIS, University of Tokyo, 4-6-1 Komaba, Meguro-ku, Tokyo 153-8505, Japan*

¶ *Department of Chemistry, Korea University, Sejong 339-700, Korea*

§ *Department of Applied Physics, The University of Tokyo, 7-3-1 Hongo, Bunkyo-ku, Tokyo 113-8656, Japan*

|| *Electrical and Computer Engineering, National University of Singapore, Singapore, Republic of Singapore 117576*

⊥ *Department of Emerging Materials Science, DGIST, 333 TechnoJungang, Hyeongpung, Daegu 42988, Korea*

# *RIKEN Center for Emergent Matter Science (CEMS), 2-1 Hirosawa, Wako, Saitama 351-0198, Japan*

@ *Institute for Nano Quantum Information Electronics, University of Tokyo, 4-6-1 Komaba, Meguro-ku, Tokyo 153-8505, Japan*

E-mail: minkyung.jung@dgist.ac.kr; jseo@dgist.ac.kr; hirakawa@iis.u-tokyo.ac.jp

Tel: +82 53 785 3501, Fax: +82 53 785 3439

## 1. TEM and EDS analysis of $Cd_3As_2$ nanowires

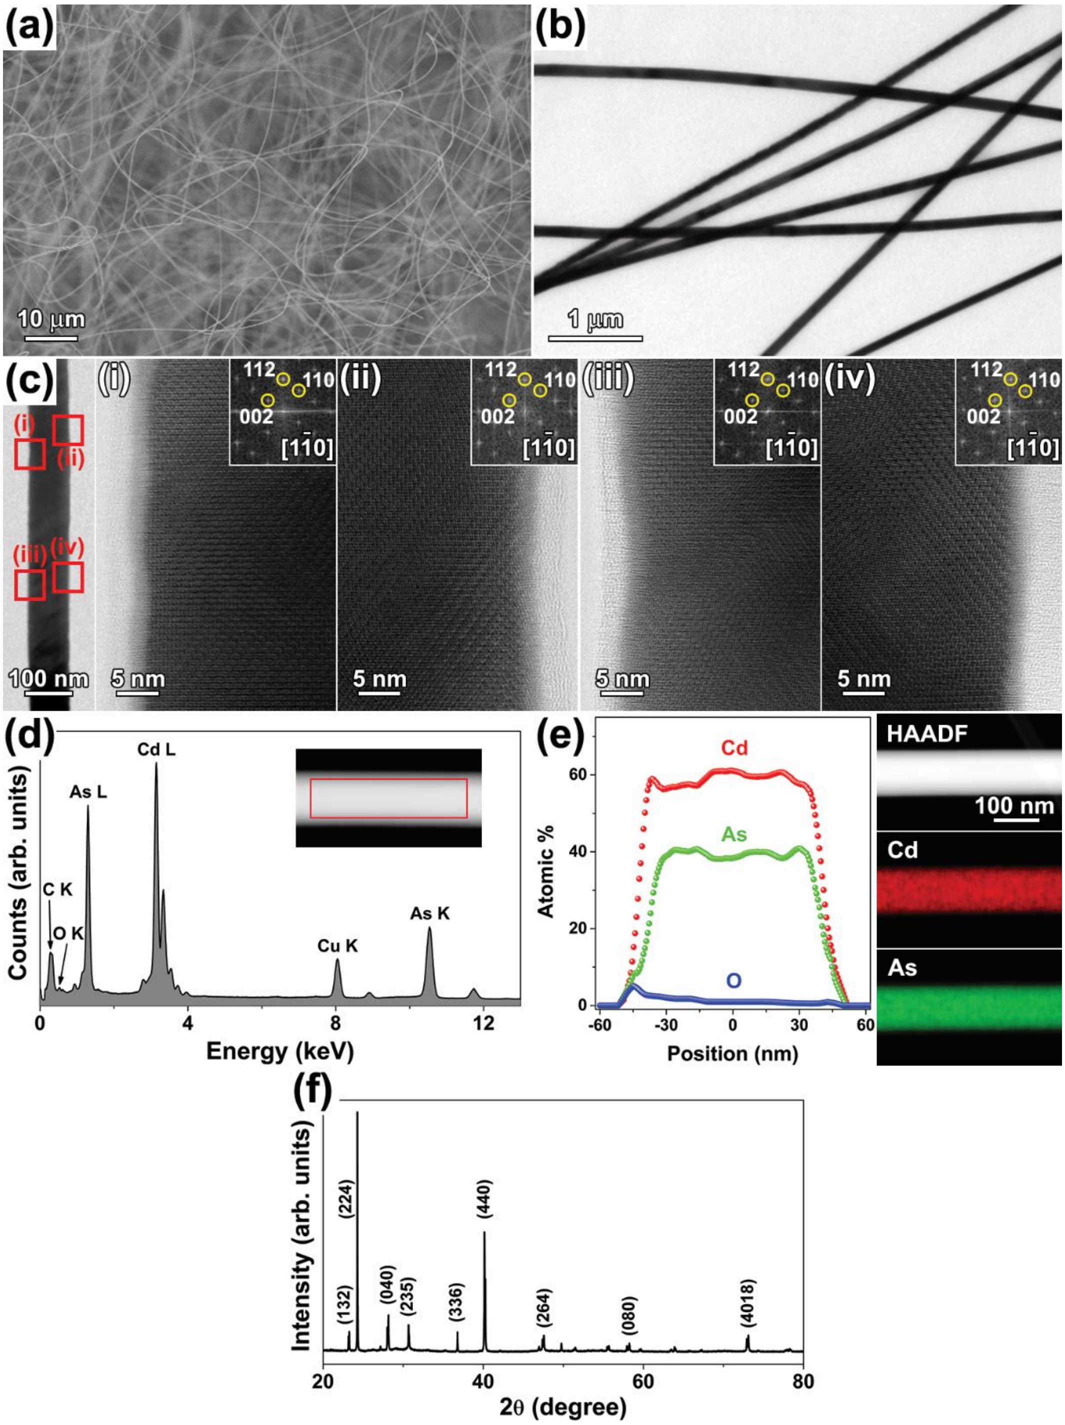


Figure S1. (a) SEM image of $Cd_3As_2$ nanowires grown on a Si substrate, and (b) high-resolution TEM (HRTEM) image, showing a general morphology of $Cd_3As_2$ nanowires. Most of them are straight and the average diameter is 80 nm. They are usually sheathed with thin amorphous layer with a thickness of 2-7 nm. (c) HRTEM images for selected $Cd_3As_2$ nanowire having smooth surface. Lattice-resolved TEM and corresponding FFT images (zone axis = [1$\bar{1}$0]) of (i)-(iv) regions show the single crystalline nature of $Cd_3As_2$ nanowire with the growth direction of [112]. The spacing between the neighboring (112) planes is 0.73 nm, which is consistent

with the reference value ($d_{211}$ = 0.731 nm; tetragonal phase with $a$ = 12.633 Å and $c$ = 25.427 Å). It indicates that the nanowires are perfectly single-crystalline over whole length, with no polycrystal domains. (d) Energy dispersive X-ray fluorescence spectroscopy (EDX) spectrum of $Cd_3As_2$ nanowire and corresponding high-angle annular dark field (HAADF) scanning TEM (STEM) image. These data were acquired using TEM (FEI Talos F200X) operated at 200 keV that equipped with high-brightness Schottky field emission electron source (X-FEG) and Super-X EDS detector system (Bruker Super-X). This EDX has powerful sensitivity and resolution in the low photon energy region. The Cd and As compositions distribute homogeneously over whole nanowire and the atomic ratio of Cd:As is 3:2 using the peaks of Cd L shell and As L shell. The O K shell peak is separated from the C K shell peak (originated from the TEM holey carbon grid), showing a negligible intensity. (e) EDX mapping (with HAADF STEM image) and line profile of Cd and As elements across the nanowire, showing the homogeneous distribution of Cd and As with a small amount of O at the shell region. (f) XRD patterns of as-grown $Cd_3As_2$ nanowires. The peaks are indexed using the reference values ($I4_1/acd$, $a$ = 12.633 Å and $c$ = 25.427 Å).[1]

## 2. Magnetoresistance and temperature dependence of resistance

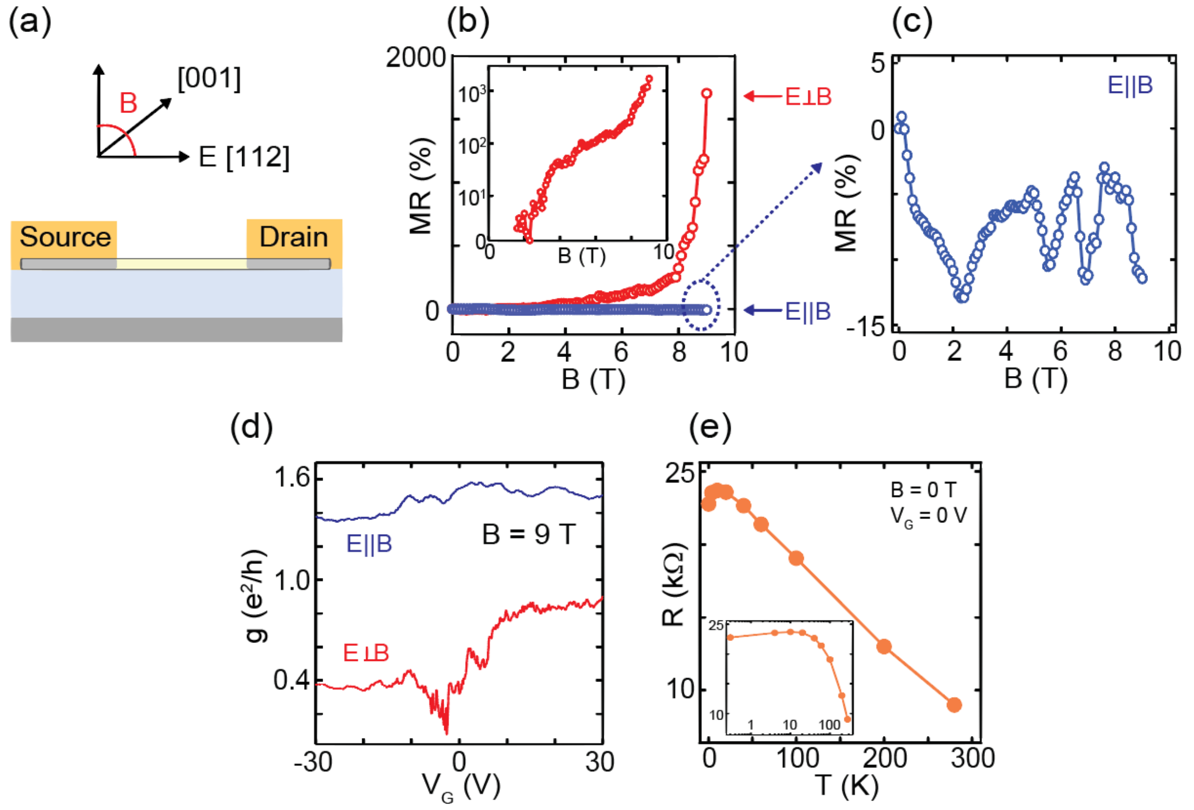


Figure S2. (a) Device schematic and electric and magnetic field directions. (b) Magnetoresistance (MR) measured at $T$ = 300 mK with the applied magnetic field perpendicular (red curve) and parallel (blue curve) to the electric field up to 9 T. The MR is defined as [R(B) – R(0)]/R(0) × 100 (%). The MR reaches a value of $1.7 \times 10^3$ (%) at $B$ = 9 T for the perpendicular field. The inset shows the MR as a function of magnetic field in a logarithmic scale. (c) The magnified plot of the MR for the parallel field in (b). The data shows the negative MR, indicative of the chiral anomaly effect in Dirac semimetals. (d) Conductance as a function of gate voltage for perpendicular (red curve) and parallel (blue curve) magnetic field to the nanowire axis. (e) Resistance as a function of temperature. Inset: Logarithmic plot.

We plot the magnetoresistance (MR) for the perpendicular (red color) and parallel (blue color) magnetic fields in Figure S2b. The MR in the perpendicular field increases dramatically as the magnetic field increases. For the parallel magnetic field to the nanowire, the NMR appears, indicative of the chiral anomaly effect in Dirac semimetals.[2] The transfer curves for the perpendicular and parallel fields ($B$ = 9 T) show clearly different behavior (Figure S2d). In the parallel field, the Coulomb oscillation is not observed, while in the perpendicular field the Coulomb oscillation is observed, as explained in the main text. This result supports our analysis that the quantum dot formation is due to magnetic barriers.

## 3. Temperature dependence of conductance

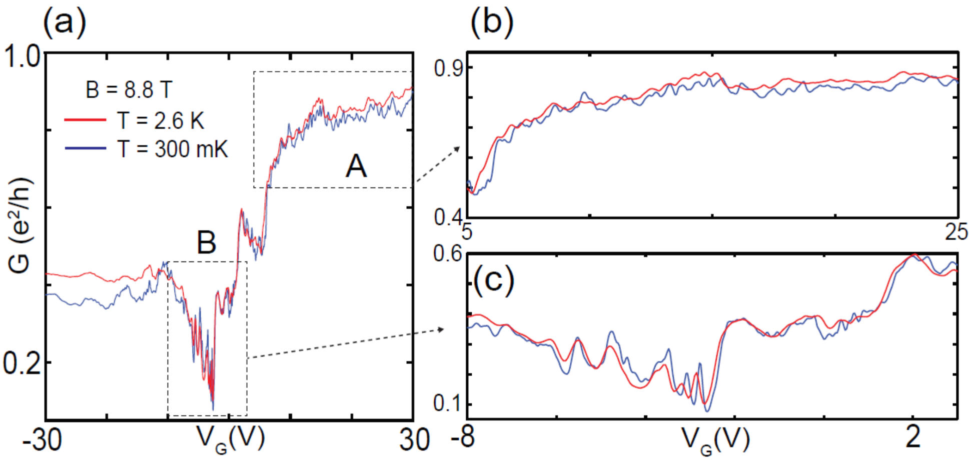


Figure S3. (a) Temperature dependence of conductance taken at $B$ = 8.8 T. (b) Magnified conductance plot of area A and (c) B. At $T$ = 2.6 K, the amplitude of universal conductance fluctuations decreases.

## 4. Calculation of transmission probability

To calculate the suppression of Klein tunneling in the presence of magnetic field, we started from the low energy Dirac Hamiltonian:

$$H = \hbar v_F \boldsymbol{k} \cdot \boldsymbol{\sigma} + V_0$$

where $V_0$ is a potential barrier at the central region of the nanowire which can be controlled by backgate voltages in the experiment, $\boldsymbol{\sigma}$ is Pauli matrix, and the wave vector $\boldsymbol{k}$ is chosen as $k_x = k_F \cos\gamma \cos\phi$, $k_y = k_F \cos\gamma \sin\phi$, $k_z = k_F \sin\gamma$ where $\gamma$ is the angle between $k_F$ and $z$-axis, $\phi$ is the azimuthal angle with respect to the $x$-axis. Application of the magnetic field along $z$-axis is modeled by introducing the vector potential $A_y = B_z x$ using Landau gauge. Thus, the transverse wave vector $k_y$ transforms as $k_y \rightarrow k_y + eA_y/\hbar$. Choosing the tunneling transmission along $k_x$, the system is translationally invariant along both transverse directions. Hence, the $k_y$ and $k_z$ are good quantum numbers. However, the momentum along the transmission direction transforms as $k_x(E_F)$ to $q_x(E_F + V_0)$ within the central region, which can be derived from the dispersion relation. The transmission probability $T(\phi, \gamma)$ is calculated by the transfer matrix method by considering three regions shown in the schematic of Figure 5a in the main text, and the result is shown in Figure 5c.

The linear increase in $A_y$ can be approximately modeled by splitting up the region under magnetic field into many short segments, each with a uniform value of $A_y$ as shown in Figure S4.

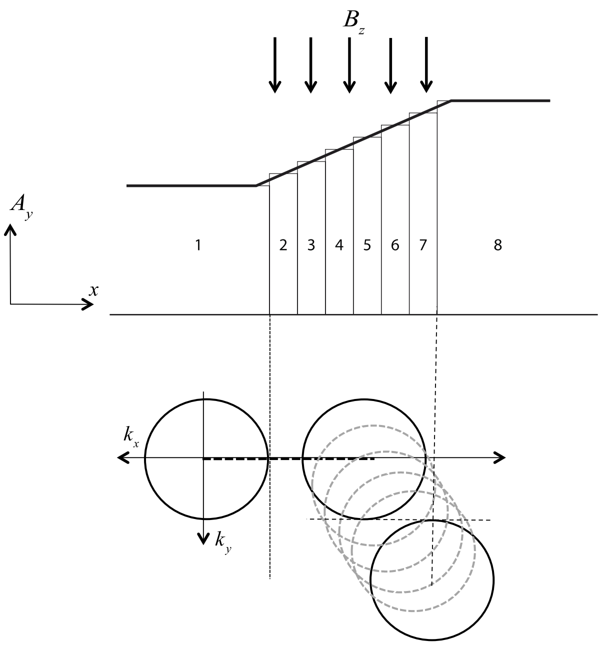


Figure S4. (Upper panel) Approximating a linear potential step as a series of short constant segments. (Lower panel) The orientation of the Fermi surfaces, which gradually shift due to the linearly increasing gauge potential $A_y$.

We briefly describe the transfer matrix approach used to calculate the transmission through the system. Consider an interface between two of the segments, say for instance the segments 1 and 2 in Figure S4. We set the *x* coordinate of the interface at 0. Matching the wavefunctions at the interface, we have the matrix equation

$$\begin{pmatrix} \mathbf{C}_+^L & \mathbf{C}_-^L & -\mathbf{C}_+^R & -\mathbf{C}_-^R \\ \mathbf{I}_{N/2} & \mathbf{0}_{N/2} & \mathbf{0}_{N/2} & \mathbf{0}_{N/2} \\ \mathbf{0}_{N/2} & \mathbf{0}_{N/2} & \mathbf{0}_{N/2} & \mathbf{I}_{N/2} \end{pmatrix} \begin{pmatrix} \mathbf{a}_+^L \\ \mathbf{a}_-^L \\ \mathbf{a}_+^R \\ \mathbf{a}_-^R \end{pmatrix} = \begin{pmatrix} \mathbf{0}_{N/2} \\ \mathbf{0}_{N/2} \\ \mathbf{a}_+^L \\ \mathbf{a}_-^R \end{pmatrix} \qquad (1)$$

where *N* generally refers to the number of degrees of freedom in the system. Specifically in Eq. (1), $N = 2$, i.e., the number of real spin degrees of freedom. $\mathbf{C}_\pm^{L/R}$ are matrices formed from the horizontal concatenation of the column vectors representing the eigen-spinors in the segments to the left and right of the interface, as indicated by the $L/R$ superscript, propagating or decaying in the $\pm x$ direction, as indicated by the $\pm$ subscript. The explicit expression for $\mathbf{C}_\pm^{L/R}$ is $\frac{1}{\sqrt{2(1-\sin(\gamma^{L/R}))}}\begin{pmatrix} \exp(-i\phi_\pm^{L/R})\cos(\gamma^{L/R}) \\ 1-\sin(\gamma^{L/R}) \end{pmatrix}$. $\mathbf{I}_{N/2}$ and $\mathbf{0}_{N/2}$ are the $(N/2 \times N/2)$ identity and zero matrices, respectively, while $\mathbf{a}_\pm^{L/R}$ are column vectors of the weightages of the eigenspinors $\pm$ in the Left/Right segment propagating/decaying in the $\pm x$ direction.

For incidence from the left / right side of the interface we can define the matrices $\mathbf{T}_{R/L}$ and $\mathbf{R}_{R/L}$. These matrices give the transmission (**T**) and reflection (**R**) coefficients for incidence from the Left / Right side of the interface as indicated by the $L/R$ subscript. Hence, for instance, $\mathbf{T}_L\boldsymbol{a}_+^L + \mathbf{R}_R\boldsymbol{a}_-^R = \boldsymbol{a}_+^R$, $\mathbf{R}_L\boldsymbol{a}_+^L + \mathbf{T}_R\boldsymbol{a}_+^R = \boldsymbol{a}_-^L$. Writing the matrix on the left hand side of Eq. (1) as **A**, we have

$$\mathbf{T}_L = \mathbf{A}^{-1}_{[2N/2+(1:N/2),2N/2+(1:N/2)]},$$

$$\mathbf{R}_L = \mathbf{A}^{-1}_{[N/2+(1:N/2),2N/2+(1:N/2)]},$$

$$\mathbf{T}_R = \mathbf{A}^{-1}_{[2N/2+(1:N/2),3N/2+(1:N/2)]},$$

$$\mathbf{R}_R = \mathbf{A}^{-1}_{[3N/2+(1:N/2),3N/2+(1:N/2)]}. \qquad (2)$$

where the subscript of the matrix constitutes sub-matrix of $\mathbf{A}^{-1}$ and $(1{:}N/2)$ is a running number series from 1 to $N/2$. These expressions hold for a single interface between two segments. The net transmission through the entire system consisting of multiple segments in Figure S4 can be obtained through an iterative process. We begin by defining $\widetilde{\mathbf{T}}^1 = \mathbf{T}_L^1$ and $\widetilde{\mathbf{R}}^1 = \mathbf{R}_L^1$, where the 1 superscript on top of $\mathbf{T}/\mathbf{R}_L^1$ indicates that these are the $\mathbf{T}/\mathbf{R}_L$ matrices obtained from Eq. (2) for the interface between segments 1 and 2, and the tilde on top of the $\widetilde{\mathbf{T}}/\widetilde{\mathbf{R}}^i$ indicates that this is the 'net' Transmission / Reflection matrix for a system consisting of segments from number 1 up to and including $i$ as depicted in Figure S4, with the ($i$+1)th segment extending to semi-infinity to the right.

Introducing the matrix $\mathbf{P}_\pm^i \equiv \text{diag}(\exp(\pm i k_\pm^i\, L^i)$, where $k_\pm^i$ is the wavevectors of the states propagating in the $\pm x$ direction in the ($i$ + 1)th segment, and $L^i$ is the length of the ($i$+1)th segment, we have

$$\widetilde{\mathbf{T}}_L^{i+1} = \mathbf{T}_L^{i+1}\left(\mathbf{I}_{N/2} - \mathbf{P}_+^i\widetilde{\mathbf{R}}_R^i\mathbf{P}_-^i\mathbf{R}_L^{i+1}\right)^{-1}\mathbf{P}_+^i\widetilde{\mathbf{T}}_L^i \qquad (3)$$

$$\widetilde{\mathbf{R}}_R^{i+1} = \mathbf{R}_R^{i+1} + \mathbf{T}_L^{i+1}\mathbf{P}_+^i\widetilde{\mathbf{R}}_R^i\left(\mathbf{I}_{N/2} - \mathbf{P}_-^i\mathbf{R}_L^{i+1}\mathbf{P}_+^i\widetilde{\mathbf{R}}_R^i\right)^{-1}\mathbf{P}_-^i\mathbf{T}_R^{i+1} \qquad (4)$$

Iteratively applying Eqs. (3) and (4) for all the $N_S$ segments in the system, we finally obtain $\widetilde{\mathbf{T}}_L^N$ which gives the transmission from the source (segment 1) to the drain (segment $N_S$).

## 5. Addition energy of quantum dot

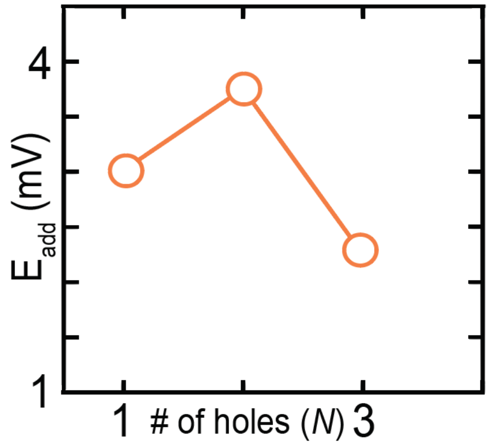


Figure S5. Addition energy $E_{add}$ as a function of hole number. $E_{add}$ is deduced from the Coulomb diamond size in Figure 6a of main text.

## 6. Temperature dependence of Coulomb stability diagram

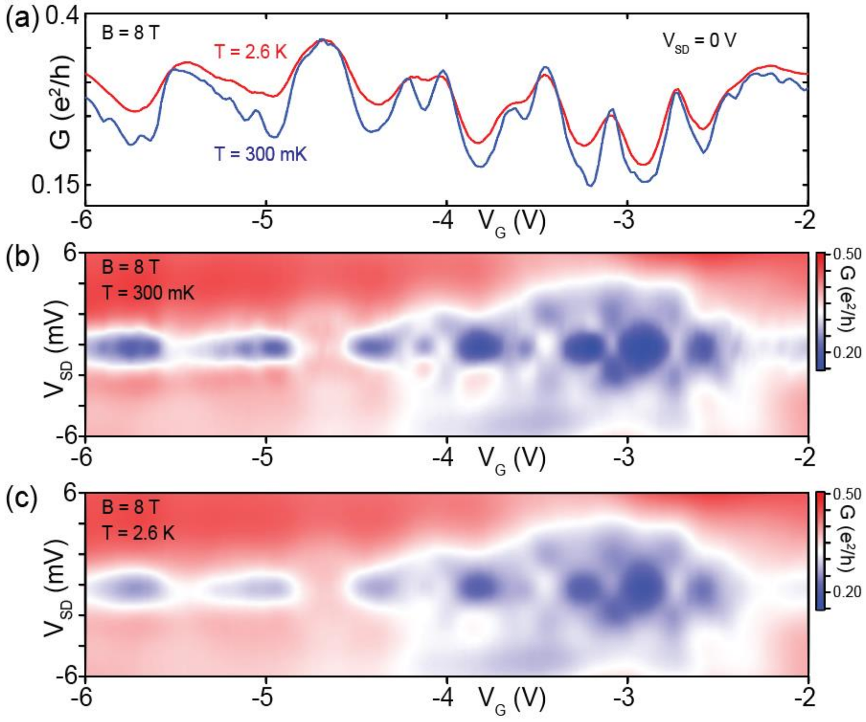


Figure S6. (a) Temperature dependence of Coulomb oscillations, (b-c) Coulomb stability diagrams measured at both $T$ = 300 mK and 2.6 K for $B$ = 8 T. As the temperature increases, the Coulomb diamonds are broadened due to thermal energy.

## 7. Fabry-Perot like interference at low magnetic field

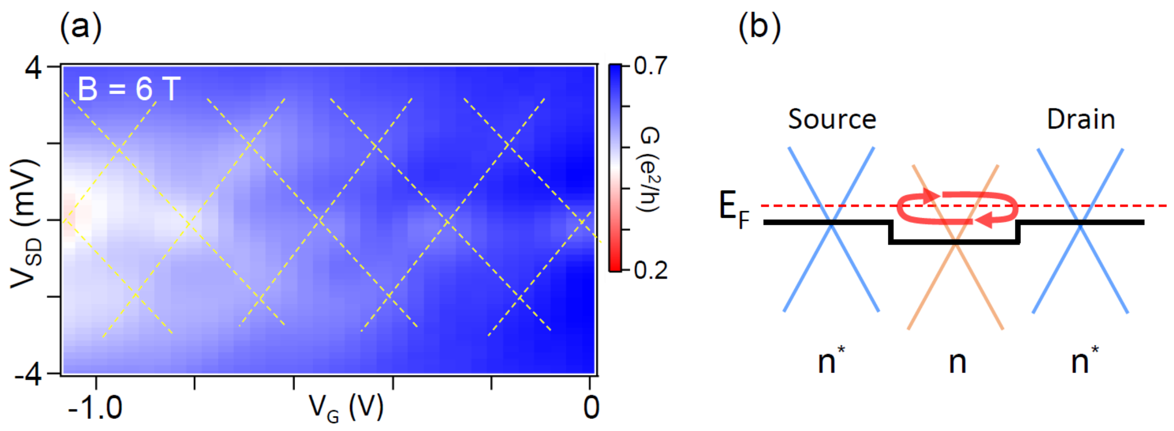


Figure S7. (a) Conductance measured in a n*–n–n* configuration as a function of $V_{SD}$ and $V_G$ at $B = 6$ T. The device shows regular checkboard patterns on the varying high conductance as marked by the dashed lines. This can be attributed to Fabry-Perot interferences caused by the impinging electron wave interfering with the reflected wave between the source and drain electrodes as shown in (b). (b) Schematic of energy diagram.

The periodic pattern at $V_{SD} = 0$ V shows a pronounced phase shift of $\pi$ at a characteristic voltage $V_C$. From the Figure S6a, we obtain $V_C \sim 2$ mV. Using the relationship between $V_C$ and the effective channel length $L$ of the Fabry-Perot resonator in the Dirac materials, $L = v_F h/2eV_C$,[3] where $v_F = 1.55 \times 10^5$ m/s is the Fermi velocity of $Cd_3As_2$ semimetal and $h$ the Planck constant,[4] we estimate $L$ to be ~ 160 nm, which is close to the device channel length measured by SEM.

References


1. Ali, M. N.; Gibson, Q.; Jeon, S.; Zhou, B. B.; Yazdani, A.; Cava, R. J. *Inorg. Chem.* **2014**, 53, 4062-4067
2. Li, H.; He, H.; Lu, H.-Z.; Zhang, H.; Liu, H.; Ma, R.; Fan, Z.; Shen, S.-Q.; Wang, J. *Nature commun*. **2016**, 7, 10301-10307.
3. Liang, W.; Bockrath, M.; Bozovic, D.; Hafner, J. H.; Tinkham, M.; Park, H. *Nature* **2001**, 411, 665-669.
4. Neupane, M.; Xu, S-Y.; Sankar, R.; Alidoust, N.; Bian, G.; Liu, C.; Belopolski, I.; Chang, T-R.; Jeng, H-T.; Lin, H.; Bansil, A.; Chou, F.; Zahid Hasan, M. *Nat. Commun.* **2014**, 5, 3786-3793.
